# Supplementary material for: Generalisation effects of predictive uncertainty estimation in deep learning for digital pathology
Source: arXiv:2112.09693 source file (2022-05-20)
Supplement: Supplementary file 1 [file 06_Appendix.tex]

%\begin{table}[]
%\begin{tabular}{|l|l|l|l|}
\begin{footnotesize}
\setlength{\LTleft}{-20cm plus -1fill}
\setlength{\LTright}{\LTleft}
\begin{longtable}{|l|l|l|l|}
%\begin{longtable}{|p|p|p|p|}
\hline
 \textbf{Method} & \textbf{Explains} & \textbf{Result representation} & \textbf{Technical approach}  \\ \hline
 Quantile Regression & Irreducible & Auxiliary measures & Frequentist techniques \\
 Forests \cite{Meinshausen2006} & uncertainty & & \\ \hline
 Conformal Prediction \cite{Papadopoulos2007}  & Reducible uncertainty & Auxiliary measures & Other techniques \\ \hline
 Activation  & Inner workings & Synthetic visualisations & Activation optimisation   \\
 maximisation \cite{Erhan2009} & & & \\ \hline
 Saliency maps \cite{Simonyan2013} & Predictions & Visualisations on the input & Back-projection to   \\ 
  &  &  & input space  \\ \hline
 DeconvNet \cite{ZeilerFergus2014} & Predictions & Synthetic visualisations & Back-projection to   \\ 
  &   &  & input space  \\ \hline
 Guided Backprop \cite{Springenberg2014} & Predictions & Synthetic visualisations & Back-projection to   \\ 
  &  of NN &  & input space  \\ \hline
 Object detectors in & Prediction; &  Visualisations on the input & Input perturbations  \\ 
 Deep Scene \cite{Zhou2014} & Inner workings &  &   \\ \hline
 Layer-wise relevance  & Predictions  & Visualisations on the input  & Back-projection to   \\ 
 propagation \cite{Bach2015} &  &  & input space   \\ \hline
 Probabilistic &  Reducible uncertainty  & Auxiliary measures & Bayesian neural  \\ 
 backpropagation \cite{Hernandez-Lobato2015} &  &  & networks \\ \hline
 Inverting Deep Image & Inner workings & Synthetic visualisations & Activation optimisation  \\ 
 Representations  \cite{Mahendran2015} &  &  &  \\ \hline
 BCNN with Bernoulli & Reducible uncertainty & Auxiliary measures & Bayesian neural\\
  approximations \cite{gal2015bayesian} & & & networks \\ \hline
 Deep visualization \cite{yosinski2015understanding} & Inner workings & Synthetic visualisations & Activation optimisation \\ \hline
 Bayes by Backprop \cite{Blundell2015} & Reducible uncertainty & Auxiliary measures & Bayesian neural \\ 
 & & & networks \\ \hline
 Bootstrapped DQN \cite{Osband2016} &  Reducible uncertainty & Auxiliary measures & Frequentist techniques \\ \hline
 Multifaceted Feature & Inner workings & Synthetic visualisations & Activation optimisation  \\ 
 Visualization \cite{Nguyen2016} &  &  &  \\ \hline
 Inverting feature & Inner workings & Synthetic visualisations & Activation optimisation\\ 
 representations \cite{Dosovitskiy2016} &  &  & \\ \hline
 Class activation  & Prediction & Visualisations on the input & Back-projection to   \\ 
 mapping (CAM) \cite{Zhou2016} &  &  & input space  \\ \hline
 Dropout as Bayesian &  Reducible uncertainty & Auxiliary measures & Bayesian   \\
 approximation \cite{Gal2016} &  &  & approximations \\ \hline
 Disco nets \cite{Bouchacourt2016} & Irreducible uncertainty & Auxiliary measures & Bayesian approximations  \\ \hline
 Deep generator &  Inner workings & Synthetic visualisations & GANs methods \\ 
 networks \cite{NguyenDosovitskiy2016} &  &  &  \\ \hline
 Distinct class & Prediction & Visualisations on the input & Back-projection to \\ 
 saliency maps \cite{Shimoda2016} &  &  & input space \\ \hline
 LIME \cite{Ribeiro2016} & Prediction & Visualisations on the input & Input perturbations \\ \hline
 Uncertainty with & Reducible uncertainty; &  Auxiliary measures & Frequentist techniques   \\
 deep ensembles \cite{Lakshminarayanan2017} & Irreducible uncertainty  &  &   \\
 & of NN & & \\ \hline
 Deep Taylor & Predictions  & Visualisations on the input  & Back-projection to   \\ 
 decomposition \cite{Montavon2017} &  &  & input space   \\ \hline
 SHAP \cite{LundbergLee2017} & Predictions & Visualisations on the input & Input perturbations \\ \hline
 PatternNet and & Predictions & Visualisations on the input & Back-projection to \\ 
 PatternAttribution \cite{Kindermans2017} &  &  & input space \\ \hline
 Integrated Gradients \cite{Sundararajan2017} & Predictions & Visualisations on the input & Back-projection to \\ 
 & & & input space \\ \hline
 Network Dissection \cite{Bau2017} & Inner workings & Showing by example & Other techniques \\ 
 & & & \\ \hline
 Grad-CAM \cite{Selvaraju2017} & Predictions & Visualisations on the input & Back-projection to \\ 
 & & & input space \\ \hline
 Uncertainties in Bayesian & Reducible uncertainty; & Auxiliary measures  & Bayesian neural  \\ 
 deep learning \cite{KendallGal2017} & Irreducible uncertainty &  & networks \\ \hline
 Meaningful  & Predictions & Visualisations on the input  & Input perturbations \\ 
 Perturbation \cite{Fong2017} & & & \\ \hline
 SmoothGrad \cite{Smilkov2017} & Predictions & Visualisations on the input & Back-projection to \\ 
 &  &  & input space \\ \hline
 Real Time Image & Predictions & Visualisations on the input & Input perturbations  \\ 
 Saliency \cite{Dabkowski2017} &  &  &   \\ \hline
 Prediction Difference &  &  &  \\ 
 Analysis \cite{Zintgraf2017} & Predictions & Visualisations on the input & Input perturbations  \\ \hline
 Influence Functions \cite{WeiKoh2017} & Predictions & Auxiliary measures & Other techniques \\ \hline
 Interpretable CNNs \cite{ZhangWuZhu2018} & Predictions & Visualisations on the input & Interpretable design  \\ \hline
 Generative Visual  &  &  &  \\ 
 Rationales \cite{Seah2018} & Predictions & Synthetic visualisations & GANs methods \\ \hline
 Weight-perturbation & Reducible uncertainty & Auxiliary measures  & Bayesian neural  \\ 
 in ADAM \cite{Khan2018} &  &  & networks \\ \hline
 Uncertainty in Bayesian & Reducible uncertainty; & Auxiliary measures & Bayesian neural \\ 
 Deep Learning \cite{Depeweg2018} & Irreducible uncertainty &  & networks \\ \hline
 Monotone composite  & Irreducible uncertainty & Auxiliary measures & Frequentist techniques  \\
 quantile regression NN \cite{Cannon2018} &  &  &  \\ \hline
 Deep k-Nearest & Predictions; & Showing by example; & Other techniques  \\ 
 Neighbors \cite{Papernot2018} & Reducible uncertainty & Auxiliary measures  &   \\ \hline
 Laplace approximation for & Reducible uncertainty & Auxiliary measures  & Bayesian approximations  \\ 
 estimating uncertainty \cite{Ritter2018} &  &  &  \\ \hline
 TCAV \cite{Kim2018} & Inner workings & Showing by example & Other techniques \\ \hline
 Bayesian uncertainty in  & Reducible uncertainty & Auxiliary measures & Bayesian approximations \\ 
 batch normalized NN \cite{Teye2018}  &  &  &  \\ \hline
 Excitation Backprop \cite{Zhang2018ExcitationBackprop} & Predictions & Visualisations on the input & Back-projection to \\
 & &  & input space \\ \hline
 Prediction Intervals for & Irreducible uncertainty & Auxiliary measures & Frequentist techniques \\ 
 Deep Learning \cite{Pearce2018PredictionIntervals}&  &  &  \\ \hline
 Bayesian Ensembling  \cite{Pearce2018BayesianEnsembling} & Reducible uncertainty & Auxiliary measures & Bayesian approximations \\ \hline
 Blocks \cite{Olah2018} & Inner workings & Synthetic visualisations & Activation optimisation \\ \hline
 Class Hierarchy &  &  &  \\
 in CNNs \cite{Alsallakh2018} & Inner workings & Showing by example & Other techniques \\ \hline
 Data augmentation for   & Irreducible uncertainty & Auxiliary measures & Input perturbations  \\
 uncertainty estimation \cite{Ayhan2018} & & & \\ \hline
 Visualization and Anomaly  & Inner workings; & & \\
 detection using t-SNE \cite{Kevin2018} & Reducible uncertainty & Showing by example & Other techniques \\ 
 &&& \\ \hline
 Uncertainty via noise & Reducible uncertainty & Auxiliary measure & Bayesian neural \\ 
 contrastive priors \cite{Hafner2019} &  &  & networks \\ \hline
 FullGrad \cite{srinivas2019fullgradient} & Prediction & Visualisations on the input & Back-projection to   \\ 
  &  &  & input space  \\ \hline
 SpRAy \cite{Lapuschkin2019} & Inner workings & Showing by example & Other techniques \\ \hline
 Influence-directed & Predictions;  & Showing by example & Other techniques \\ 
 explanations \cite{Leino2019} & Inner workings  &  &  \\ \hline
 Bayesian CNN with & Reducible uncertainty & Auxiliary measures & Bayesian neural\\
 variational inference \cite{shridhar2019comprehensive} & & & networks \\ \hline
 Uncertainty quantification & Reducible uncertainty; & Auxiliary measures & Bayesian neural  \\ 
 in Bayesian NN \cite{Kwon2020} & Irreducible uncertainty &  & networks  \\ \hline
 Dissecting the weight & Inner workings & Auxiliary measures & Other techniques \\
 space of NN \cite{Eilertsen2020} & & & \\ \hline

%\end{tabular}
%\captionsetup{margin=-14pt}
\caption{List of methods and their categorisations, ordered by the year of publishing.} \label{tab:methods_cats}
%\end{table}
\end{longtable}
\end{footnotesize}
